# Supplementary material for: Learning What to Learn for Video Object Segmentation
Source: arXiv:2003.11540 source file (2020-05-01)
Supplement: Supplementary file 1 [file complexity.tex]

\section{Computational Complexity}

%-$\sum_t x_t \conv \targetparam$  num operations: $H \times W \times C \times D \times K \times K \times \text{num samples} \times N$ \\
%-$\sum_t x_t \conv\tp r$ num operations $H \times W \times C \times D \times K \times K \times \text{num samples} \times N$?\\
%-$\sum_t sx_t \conv g$\\ 

Here, we analyze the computational complexity of our internal few-shot learner. The main computational cost in our few-shot learner is the computation of the gradient $g$ step-length $\alpha$ in each steepest-descent iteration \eqref{eq:sd-steplength}. This operation is dominated by the convolutions $x_t \conv \targetparam$, $x_t \conv g^i$, and the transposed convolution $[x_t\conv\tp]$, each of which scale linearly with the feature map size $H \times W \times C$, the kernel size $K \times K$, the number of mask encoding channels $D$, and the size of the training set $M$. Thus the few-shot learner has a complexity  $\mathcal{O}(HWK^2CDMN_\text{SD})$, where $N_\text{SD}$ is the number of steepest-descent iterations employed.

% In comparison, computing the closed form solution $\targetparamvec=X\tp W(X W X\tp W\tp + I\lambda)^{-1} e$ requires computing $X_t W_t X_t\tp W_t\tp \in reals^{HWD\times HWD}$, computing $X\tp W$ requires a point-wise operation with $W$ and $[x_t \conv\tp]$, $V = (X W X\tp W\tp + I\lambda)^{-1}$ has complexity $ \mathcal{O}(N^3)$ with $N=HW$. Further, $V_t e$ requires computing $v_t \conv \labelenc$.  

We compare the complexity of our few-shot learner with the complexity of computing the closed-form solution of our optimization problem \eqref{eq:L2_mat}. We use the matrix formulation of the internal loss \eqref{eq:L2_mat}, setting $X = [X_1\tp, \ldots, X_M\tp]\tp \in \reals^{HWDM \times K^2CD}$, $W=\diag \big([\vecop( \weightpredictor(\maskgt_1))\tp, \ldots, \vecop( \weightpredictor(\maskgt_M))\tp]\big) \in \reals^{HWDM \times HWDM}$ and $e = [e_1\tp, \ldots, e_M\tp]\tp \in \reals^{HWDM}$. Thus, the loss can be written as,
\begin{equation}
    L(\targetparamvec)= \frac{1}{2}\big\|W (X \targetparamvec - e)\big\|^2 +  \frac{\lambda}{2}\big\|\targetparamvec\big\|^2\,.
    \label{eq:L2_matmat}
\end{equation}
The primal closed form solution is obtained as follows,
\begin{align}
&\nabla L = 0 \iff \\
&X\tp W^2(X \targetparamvec -e) + \lambda \targetparamvec = 0 \iff \\
&\targetparamvec = (X\tp W^2X + \lambda I)^{-1}X\tp W^2 e\,,
\label{eq:closed_form}
\end{align}
Note that \eqref{eq:closed_form} can be solved independently for each of the $D$ output dimensions. We can therefore assume $D=1$ in \eqref{eq:closed_form} and add the linear scaling in $D$ as the final step.  We observe that the computation of the closed-form solution \eqref{eq:closed_form} is dominated by the matrix multiplications,  $(XW)\tp  XW$, where $XW \in \reals^{HWM \times K^2C}$ and of solving the linear system in \eqref{eq:closed_form}. The latter has a dimensionality of $K^2C$, resulting in a $\mathcal{O}(K^6C^3)$ complexity. The matrix multiplication $(XW)\tp  XW$ has complexity $\mathcal{O}(K^4C^2HWM)$. The final complexity of the primal closed-form solution is thus $\mathcal{O}(DK^6C^3 + DK^4C^2HWM)$

\begin{table}[t!]
\caption{}\vspace{0mm}
\centering
\resizebox{\columnwidth}{!}{%
\begin{tabular}{lc}
\toprule
&\\
\midrule
Ours&$HWK^2CDMN_\text{SD}$\\
Primal Closed-form&$DK^6C^3 + DK^4C^2HWM$\\
Dual Closed-form&$H^3W^3M^3 + K^2CH^2W^2M^2$\\
\bottomrule
\end{tabular}
}\vspace{0mm}
\label{tab:complexity}
\end{table}
%$(X\tp W^2X + \lambda I) \in \reals^{K^2CD \times K^2CD}$. Due to the block diagonal nature of $X$, this reduces to $MD$ sub-computations, each with complexity $\mathcal{O}(K^4C^2HW) + \mathcal{O}(K^6C^3D^3)$. Here, $\mathcal{O}(K^4C^2HW)$ is the complexity of the matrix multiplication while $\mathcal{O}(K^6C^3)$ is the complexity of the matrix inversion. Thus the overall complexity for computing the closed-form solution is $\mathcal{O}(K^4C^2HWMD) + \mathcal{O}(K^6C^3MD)$. Compared to our few-shot learner, the matrix multiplication step in the closed-form solution has a quadratic dependency on the number of convolution kernel elements $K^C$. While the few-shot learner complexity has an additional scaling factor in the number of iterations $N_\text{SD}$, this factor is usually much smaller compared to the term $K^2C$ ($20$ as opposed to $512 \times 3^2$ in our case). 

%In our case, the few-shot learner operates on feature maps with channel dimension $C=512$, 

Another alternative is to use the  dual form solution to the problem in \eqref{eq:L2_matmat}. We employ the Woodbury matrix formula~\cite{colquhoun1995q} to obtain the dual solution,
\begin{equation}
\label{eq:closed_form_dual}
    \targetparamvec = X\tp W(WXX\tp W+ \lambda I)^{-1} W e
\end{equation}
Similar to the primal form, the dual solution \eqref{eq:closed_form_dual} can be reduced to $D$ sub-computations. Solving the linear system leads to a complexity of $\mathcal{O}(H^3W^3M^3)$. The  matrix multiplication $WXX\tp W$ requires $\mathcal{O}(K^2CH^2W^2M^2)$ operations. The total complexity is thus  $\mathcal{O}(DH^3W^3M^3 + DK^2CH^2W^2M^2)$. The computational complexities of all three methods are summarized in Table~\ref{tab:complexities}.
