# Supplementary material for: Learning What to Learn for Video Object Segmentation
Source: arXiv:2003.11540 source file (2020-05-01)
Supplement: Supplementary file 2 [file jjval.tex]

d82a0aa15b, 691a111e7c, 97ab569ff3, d4a607ad81, f46c364dca, 4743bb84a7,  
1295e19071, 267964ee57, df59cfd91d, c557b69fbf, 927647fe08, 88f345941b, 
8ea6687ab0, 444aa274e7, ae93214fe6, b6e9ec577f, de30990a51, acb73e4297, 
6cccc985e0, ebc4ec32e6, f34a56525e, 2b351bfd7d, a43299e362, 733798921e, 
feda5ad1c2, 103f501680, da5d78b9d1, 634058dda0, 34d1b37101, 73c6ae7711, 
a8f78125b9, e1495354e4, 4fa9c30a45, c3457af795, fe3c02699d, 878a299541, 
a1193d6490, d69967143e, d6917db4be, bda224cb25, 621584cffe, 7a5f46198d,  
35195a56a1, 204a90d81f, e0de82caa7, 8c3015cccb, 4e3f346aa5, 5e418b25f9, 
4444753edd, c7bf937af5, 4da0d00b55, 48812cf33e, 35c6235b8d, 60c61cc2e5, 
9002761b41, 13ae097e20, ec193e1a01, d3987b2930, 72f04f1a38, 97e59f09fa, 
d0ab39112e, 9533fc037c, 2b88561cf2, 6c4387daf5, e1d26d35be, 0cfe974a89, 
0eefca067f, 887a93b198, 4bc8c676bb, 6f49f522ef, a9c9c1517e, 8dcfb878a8, 
1471274fa7, 53cad8e44a, 46146dfd39, 666b660284, 51e85b347b, ec3d4fac00, 
1c72b04b56, 2ba621c750, d123d674c1, bd0e9ed437, dd61d903df, 80c4a94706, 
b4d0c90bf4, 52c8ec0373, 7bc7761b8c, 25f97e926f, e72a7d7b0b, 9f913803e9, 
8bf84e7d45, a9cbf9c41b, 7abdff3086, ae13ee3d70, a68259572b, 081ae4fa44, 
8d064b29e2, 41dab05200, 6024888af8, 5110dc72c0, b0dd580a89, 2ff7f5744f, 
45c36a9eab, ec4186ce12, 72cac683e4, c2a35c1cda, 11485838c2, 5675d78833, 
55c1764e90, bfd8f6e6c9, 7ecd1f0c69, 90c7a87887, 4f414dd6e7, 211bc5d102, 
3299ae3116, 827cf4f886, 5665c024cb, 08aa2705d5, 8e1848197c, d7bb6b37a7, 
9d01f08ec6, fad633fbe1, 11ce6f452e, 644bad9729, ae3bc4a0ef, b2ce7699e3, 
f7e0c9bb83, 52c7a3d653, 7806308f33, fed208bfca, 9198cfb4ea, 8c469815cf, 
731b825695, c52bce43db, 0d2fcc0dcd, 1917b209f2, b274456ce1, d44e6acd1d, 
7e0cd25696, 8909bde9ab, 68ea4a8c3d, 69ea9c09d1, 5a4a785006, b73867d769, 
f0c34e1213, 84044f37f3, 479f5d7ef6, 3cc37fd487, f8fcb6a78c, f0ad38da27, 
d0c65e9e95, 3b6c7988f6, f9ae3d98b7, e4d4872dab, 14dae0dc93, 86a40b655d, 
4eb6fc23a2, 15617297cc, 4b67aa9ef6, 3e7d2aeb07, 4ea77bfd15, 2719b742ab, 
f04cf99ee6, 75285a7eb1, 74ef677020, c9b3a8fbda, 62d6ece152, 536096501f, 
3355e056eb, 6a48e4aea8, 04259896e2, 189ac8208a, ba98512f97, 223bd973ab, 
a3f51855c3, 8b4fb018b7, 0ea68d418b, 6d4bf200ad, c130c3fc0c, 8a31f7bca5, 
f8b4ac12f1, f85796a921, ef45ce3035, e4f8e5f46e, d5b6c6d94a, c760eeb8b3, 
0b9d012be8, 1f4ec0563d, 2df005b843, dc32a44804, 1cada35274, 4cfdd73249, 
b8f34cf72e, 53af427bb2, 1329409f2a, 1b8680f8cd, 2bbde474ef, 2f5b0c89b1, 
6693a52081, 684bcd8812, e1f14510fa, 72a810a799, 70c3e97e41, 7c4ec17eff, 
8a75ad7924, fd77828200, 53d9c45013, 968c41829e, d39934abe3, 6e1a21ba55, 
bc4f71372d, 57246af7d1, f49e4866ac, 1e1a18c45a, a14ef483ff, d92532c7b2, 
aab33f0e2a, f3325c3338, 4cf5bc3e60, c98b6fe013, 619812a1a7, f8c8de2764, 
6dd2827fbb, f277c7a6a4, 1ca240fede, 16e8599e94, b554843889, df0638b0a0, 
d664c89912, c5ab1f09c8, d38d1679e2, 31bbd0d793, b24fe36b2a, c1c830a735, 
75504539c3, a74b9ca19c, c6bb6d2d5c, 99dc8bb20b, 92c46be756, 7a626ec98d, 
0891ac2eb6, 7f54132e48, c47d551843, 4122aba5f9, 5aeb95cc7d, 8ca1af9f3c, 
4019231330, 8f320d0e09, 5851739c15, b69926d9fa, b132a53086, 135625b53d, 
05d7715782, e3e4134877, d3069da8bb, 747c44785c, 59a6459751, 5a75f7a1cf, 
63936d7de5, d301ca58cc, 9c404cac0c, 78613981ed, d072fda75b, 390c51b987, 
571ca79c71, 67cfbff9b1, 7a8b5456ca, efe5ac6901, c4571bedc8, 57a344ab1a, 
d205e3cff5, 39befd99fb, 3b23792b84, 6a5de0535f, ced7705ab2, 06ce2b51fb, 
dd415df125, 2f710f66bd, 0f6c2163de, e470345ede, 6b2261888d, 6671643f31, 
de74a601d3, f14c18cf6a, f38e5aa5b4, 57427393e9, 6da21f5c91, 738e5a0a14, 
0f2ab8b1ff, 4a4b50571c, a263ce8a87, 031ccc99b1, ab45078265, 01e64dd36a, 
e0c478f775, b5b9da5364, 72acb8cdf6, c922365dd4, df11931ffe, ad3fada9d9
