# Supplementary material for: Learning What to Learn for Video Object Segmentation
Source: arXiv:2003.11540 source file (2020-05-01)
Supplement: Supplementary file 3 [file davis_video_list.tex]

bike-packing, blackswan, bmx-trees, dance-twirl, 
drift-chicane, drift-straight, goat, horsejump-high, 
judo, kite-surf, motocross-jump, soapbox
