# Supplementary material for: Learning What to Learn for Video Object Segmentation
Source: arXiv:2003.11540 source file (2020-05-01)
Supplement: Supplementary file 4 [file ablation_seqtraining.tex]

\centering
\begin{tabular}{l@{~~~~}c}
\toprule
 & $\mathcal{J} (\%)$ \\
\midrule
Sequence training&79.8 \\
Pair training&79.5 \\
\bottomrule
\end{tabular}
