# Supplementary material for: Learning What to Learn for Video Object Segmentation
Source: arXiv:2003.11540 source file (2020-05-01)
Supplement: Supplementary file 5 [file ablation_sup.tex]

\centering
\begin{tabular}{l@{~~~~} (\%)c}
\toprule
 & $\mathcal{J}$ \\
\midrule
Ours&79.8 \\
ImageNet weights&78.6\\
BCE Loss&79.2 \\
Backbone Fine-tune&81.2 \\
\bottomrule
\end{tabular}
