# Supplementary material for: Learning What to Learn for Video Object Segmentation
Source: arXiv:2003.11540 source file (2020-05-01)
Supplement: Supplementary file 6 [file complexity.tex]

\begin{tabular}{lc}
\toprule
&\\
\midrule
Ours&$HWK^2CDMN_\text{SD}$\\
Primal Closed-form&$DK^6C^3 + DK^4C^2HWM$\\
Dual Closed-form&$H^3W^3M^3 + K^2CH^2W^2M^2$\\
\bottomrule
\end{tabular}
