# Supplementary material for: Learning What to Learn for Video Object Segmentation
Source: arXiv:2003.11540 source file (2020-05-01)
Supplement: Supplementary file 7 [file yvos_video_list.tex]

00f88c4f0a, 30fe0ed0ce, 39bce09d8d, 3f99366076, 63a68c6741, 67e397b1f2, 
6a75316e99, 77bec90101, 7fb4f14054, 8e2e5af6a8, 9a38b8e463, 9c693f291b, 
9ce299a510, 9fd2d2782b
